# Supplementary material for: QRFA: A Data-Driven Model of Information-Seeking Dialogues
Source: arXiv:1812.10720 source file (2018-12-27)
Supplement: Supplementary file 1 [file table.tex]

\documentclass[11pt,a4paper]{article}
\usepackage[hyperref]{emnlp2018}
\usepackage{times}
\usepackage{latexsym}
\usepackage{todonotes}

\usepackage{cleveref}
\usepackage{url}
\usepackage{multirow}

\usepackage{pdflscape}
\usepackage{afterpage}
\usepackage{capt-of}% or use the larger `caption` package
\usepackage[pass]{geometry} 
% To create good-looking book-style tables
\usepackage{booktabs}
% For resizing tables
\usepackage{adjustbox}

%\aclfinalcopy % Uncomment this line for the final submission
 %  Enter the acl Paper ID here

%\setlength\titlebox{5cm}
% You can expand the titlebox if you need extra space
% to show all the authors. Please do not make the titlebox
% smaller than 5cm (the original size); we will check this
% in the camera-ready version and ask you to change it back.

% \title{Repairing the Functional Model of Information-Seeking Dialogues} 
\title{QRFA: Data-Driven Model of Information-Seeking Dialogues}
% \title{}

\author{First Author \\
  Affiliation / Address line 1 \\
  Affiliation / Address line 2 \\
  Affiliation / Address line 3 \\
  {\tt email@domain} \\\And
  Second Author \\
  Affiliation / Address line 1 \\
  Affiliation / Address line 2 \\
  Affiliation / Address line 3 \\
  {\tt email@domain} \\}

\date{}

%
%%%%%%%%%%%%%%%%%%%%%%%%%%%%%%%%%%%%%%%%%%%%%%%%%%%%%%%%%%%%%%%%
% LaTeX handling, dirty tricks, and more
%%%%%%%%%%%%%%%%%%%%%%%%%%%%%%%%%%%%%%%%%%%%%%%%%%%%%%%%%%%%%%%%
%
\input{addon/commands}
\graphicspath{{figures/}}

%%%%%%%%%%%%%%%%%%%%%%%%%%%%%%%%%%%%%%%%%%%%%%%%%%%%%%%%%%%%%%%%
% Main matter
%%%%%%%%%%%%%%%%%%%%%%%%%%%%%%%%%%%%%%%%%%%%%%%%%%%%%%%%%%%%%%%%
%

\begin{document}

% Please add the following required packages to your document preamble:
% \usepackage{multirow}
\begin{table}[]
\centering
\caption{My caption}
\label{my-label}
\begin{tabular}{|l|l|l|l|l|l|l|l|l|l|}
\hline
\multicolumn{1}{|c|}{\multirow{3}{*}{Model/Dataset}} & \multicolumn{4}{c|}{User}                                                                                                      & \multicolumn{5}{c|}{Agent}                                                                                                                                           \\ \cline{2-10} 
\multicolumn{1}{|c|}{}                               & \multicolumn{2}{c|}{Query}                                     & \multicolumn{2}{c|}{Feedback}                                 & \multicolumn{2}{c|}{Request}                                 & \multicolumn{3}{c|}{Answer (Response)}                                                                \\ \cline{2-10} 
\multicolumn{1}{|c|}{}                               & \multicolumn{1}{c|}{Information} & \multicolumn{1}{c|}{Prompt} & \multicolumn{1}{c|}{Positive} & \multicolumn{1}{c|}{Negative} & \multicolumn{1}{c|}{Offer} & \multicolumn{1}{c|}{Understand} & \multicolumn{1}{c|}{Results}        & \multicolumn{1}{c|}{Backchannel} & \multicolumn{1}{c|}{Empty}   \\ \hline
COR                                                  & request                          & withdraw                    & accept                        & reject                        & offer                      &                                 & assert                              & promise                          & reject                       \\ \hline
                                                     &                                  &                             & be contented                  & be discontented               & withdraw                   &                                 &                                     &                                  &                              \\ \hline
                                                     & \multicolumn{9}{c|}{11 utterance labels}                                                                                                                                                                                                                                                              \\ \hline
CS                                                   & rt                               &                             & rr                            &                               & a0                         &                                 & a1i                                 &                                  &                              \\ \hline
                                                     &                                  &                             & rp                            &                               & a1p                        &                                 & a2+i                                &                                  &                              \\ \hline
                                                     &                                  &                             & rnp                           &                               & a2+p                       &                                 &                                     &                                  &                              \\ \hline
                                                     &                                  &                             &                               & rc                            &                            &                                 &                                     &                                  &                              \\ \hline
                                                     & \multicolumn{9}{c|}{10 utterance labels}                                                                                                                                                                                                                                                              \\ \hline
SCS                                                  & Initial information request      & SERP information request    & Confirms                      &                               & Query refinement offer     &                                 & SERP without modification           & Confirms                         &                              \\ \hline
                                                     & Intent clarification             &                             &                               &                               &                            & Asks to repeat                  & SERP with modification              &                                  &                              \\ \hline
                                                     & Query repeat                     &                             &                               &                               &                            &                                 & SERP with modification + Suggestion &                                  &                              \\ \hline
                                                     & Query embellishment              &                             &                               &                               &                            &                                 & Scanning document theme             &                                  &                              \\ \hline
                                                     & \multicolumn{9}{c|}{13 utterance labels}                                                                                                                                                                                                                                                              \\ \hline
ODE                                                  & set(keywords)                    & question(data)              & confirm()                     & reject()                      & list(keywords)             & prompt(keywords)                & bool(data)                          & confirm()                        &                              \\ \hline
                                                     &                                  & more()                      & success()                     &                               & prompt(link)               & verify()                        & count(data)                         & success()                        &                              \\ \hline
                                                     &                                  & prompt(link)                &                               &                               &                            &                                 & top(keywords)                       &                                  &                              \\ \hline
                                                     &                                  & verify()                    &                               &                               &                            &                                 & link(dataset)                       &                                  &                              \\ \hline
                                                     & \multicolumn{9}{c|}{17 utterance labels}                                                                                                                                                                                                                                                              \\ \hline
DSTC1                                                & inform                           & restart                     & affirm                        & negate                        & request                    &                                 & schedule                            & ack                              & sorry                        \\ \hline
                                                     & nextbus                          & repeat                      &                               &                               & open-request               & are-you-there                   & morebuses                           & hold-on                          & canthelp.cant\_find\_stop    \\ \hline
                                                     & prevbus                          & tellchoices                 &                               &                               & example                    & bebrief                         &                                     & impl-conf                        & canthelp.from\_equals\_to    \\ \hline
                                                     &                                  & goback                      &                               &                               &                            & expl-conf                       &                                     &                                  & canthelp.no\_buses\_at\_time \\ \hline
                                                     &                                  &                             &                               &                               &                            & please-repeat                   &                                     &                                  & canthelp.no\_connection      \\ \hline
                                                     &                                  &                             &                               &                               &                            & please-rephrase                 &                                     &                                  & canthelp.nonextbus           \\ \hline
                                                     &                                  &                             &                               &                               &                            &                                 &                                     &                                  & canthelp.route\_doesnt\_run  \\ \hline
                                                     &                                  &                             &                               &                               &                            &                                 &                                     &                                  & canthelp.system\_error       \\ \hline
                                                     &                                  &                             &                               &                               &                            &                                 &                                     &                                  & canthelp.uncovered\_route    \\ \hline
                                                     &                                  &                             &                               &                               &                            &                                 &                                     &                                  & canthelp.uncovered\_stop     \\ \hline
                                                     & \multicolumn{9}{c|}{32 utterance labels}                                                                                                                                                                                                                                                              \\ \hline
DSTC2                                                & inform                           &                             & ack                           & negate                        & request                    &                                 & inform                              & impl-conf                        & canthelp                     \\ \hline
                                                     & request                          &                             & affirm                        &                               & welcomemsg                 & expl-conf                       & offer                               &                                  & canthelp.exception           \\ \hline
                                                     & confirm                          &                             & thankyou                      &                               & reqmore                    & repeat                          &                                     &                                  &                              \\ \hline
                                                     & deny                             &                             &                               &                               & select                     & confirm-domain                  &                                     &                                  &                              \\ \hline
                                                     & repeat                           &                             &                               &                               &                            &                                 &                                     &                                  &                              \\ \hline
                                                     & reqalts                          &                             &                               &                               &                            &                                 &                                     &                                  &                              \\ \hline
                                                     & \multicolumn{9}{c|}{22 utterance labels}                                                                                                                                                                                                                                                              \\ \hline
\end{tabular}
\end{table}
\end{document}
